# Supplementary material for: ExSum: From Local Explanations to Model Understanding
Source: arXiv:2205.00130 source file (2022-04-30)
Supplement: Supplementary file 1 [file 2gui.tex]

\subsection{Overview}

The graphical user interface is implemented as a local Python Flask application \citep{grinberg2018flask}. In other words, it is an offline software, does not require Internet access, and does not send data to or receive data from anywhere. We design it as a web application to ensure easy and maximal compatibility across platforms. We use the Google Chrome browser for all screenshots in the paper. For installations of the server package, instructions to run it and examples, please refer to the README in the accompanying code repository.  

\begin{figure}[!htb]
    \centering
    \includegraphics[width=\textwidth]{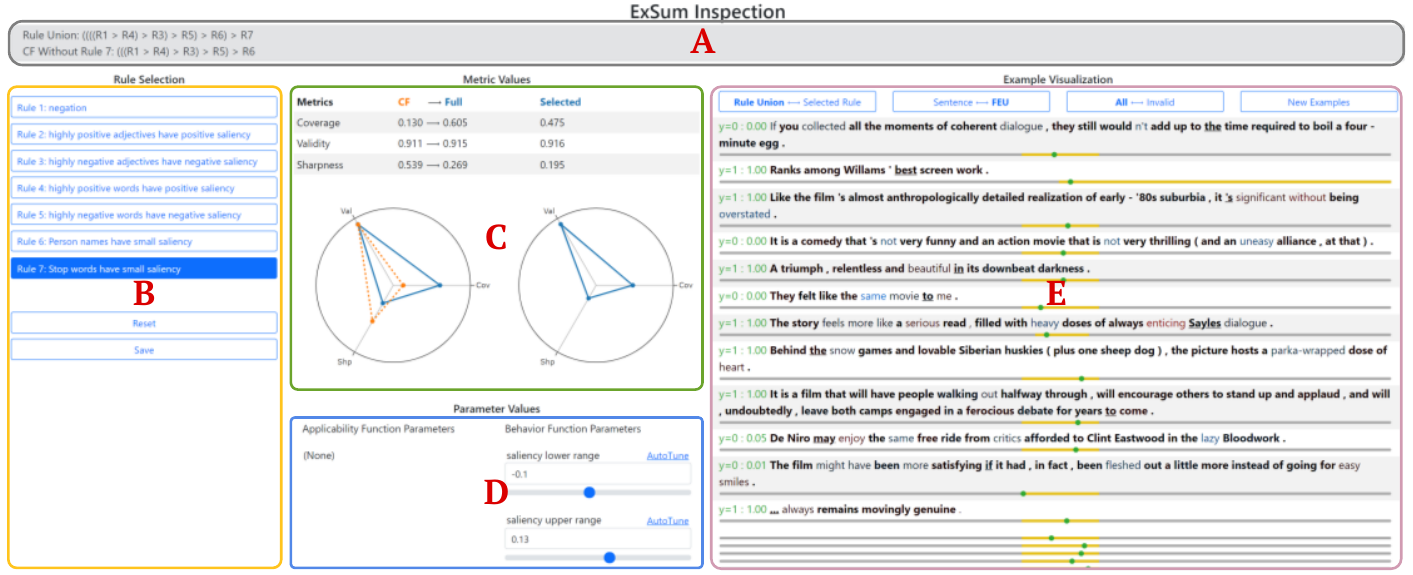}
    \caption{The graphical user interface}
    \label{fig:gui-boxed}
\end{figure}

\noindent The GUI is designed to visualize and modify one \modelname{} rule union, which is defined by its constituent rules and the composition structure. It has 5 panels. 

\subsection{Panel A}
Panel A presents the composition structure of a rule. In addition, if a rule is selected for detailed inspection, it will also show a \textit{counterfactual} (CF) rule union without the selected rule. For the screenshot shown in Fig.~\ref{fig:gui-boxed}, there are 7 rules, with the last one selected. The text in the box reads

\begin{Verbatim}[fontfamily=cmtt]
Rule Union: ((((R1 > R4) > R3) > R5) > R6) > R7)
CF Without Rule 7: (((R1 > R4) > R3) > R5) > R6)
\end{Verbatim}

\subsection{Panel B}
Panel B lists each constituent rule as a button. Fig.~\ref{fig:gui-B} shows an enlarged version of some buttons. Clicking on a button selects the corresponding rule for detailed inspection. In addition, there are two control buttons. ``Reset'' rolls back changes to the parameter values for all rules and ``Save'' writes the current parameter values for all rules to disk. 

\begin{figure}[!htb]
    \centering
    \includegraphics[width=0.4\textwidth]{figures/gui_B.png}
    \caption{An enlarged view of some buttons in panel B, with Rule 7 currently selected. }
    \label{fig:gui-B}
\end{figure}

\subsection{Panel C}
Panel C shows the metric values in both numerical and graphical formats. Fig.~\ref{fig:gui-C} shows an enlarged version of it. When a rule is selected, as in the case being visualized, the three sets of metric values are computed: full rule union, the counterfactual rule union, and the selected rule. The first two sets are visualized in the left column, in blue and orange respectively. The metric values for the selected rule is visualized on the right. They are computed only on FEUs for which the selected rule is effective. For example, the values for the lowest-precedence catch-all rule is computed on FEUs that none of the earlier rules apply, rather than on all instances. The metric values for the CF rule union and selected rule help the user effectively gauge the contribution of the selected rule and modify it if necessary. 

\begin{figure}[!htb]
    \centering
    \includegraphics[width=0.6\textwidth]{figures/gui_C.png}
    \caption{An enlarged view of panel C, with Rule 7 currently selected. }
    \label{fig:gui-C}
\end{figure}

\subsection{Panel D}
Panel D shows the parameter values for the applicability and behavior functions of the rule. Fig.~\ref{fig:gui-D} shows an enlarged version of it. While, in theory, the set of parameters can be any set, the GUI supports a continuous interval (i.e. a segment of the real number line) for a parameter value. For each parameter, the user can modify it either manually with the input field or the slider, or automatically via the automatic parameter tuning functionality, described below. For the selected Rule 7 on stop words, the applicability function is based on a list of part-of-speech check, so it does not have any numeric parameters. The behavior function specifies a constant range for the saliency value, which is parametrized by the lower bound and upper bound, both are parameters that can be modified, as shown in Fig.~\ref{fig:gui-D}. After any parameter is updated, all metric values are recomputed and updated without user intervention. 

\begin{figure}[!htb]
    \centering
    \includegraphics[width=0.7\textwidth]{figures/gui_D.png}
    \caption{An enlarged view of panel D, with parameters for Rule 7 shown. }
    \label{fig:gui-D}
\end{figure}

\noindent To automatically tune a parameter, the user can click the \ul{AutoTune} link, which brings up a pop-up, as shown in Fig.~\ref{fig:gui-autotune}. There are two search methods, linear and binary. Both modes starts at the \Verb[fontfamily=cmtt]+start value+ and aim to find a feasible value between the \Verb[fontfamily=cmtt]+start value+ and the \Verb[fontfamily=cmtt]+stop value+. Linear search moves in increment of \Verb[fontfamily=cmtt]+precision+,  while binary search stops when the halving length is less than it. A parameter value is feasible when the \Verb[fontfamily=cmtt]+target metric+ (e.g. selected rule validity as shown) reaches the specified \Verb[fontfamily=cmtt]+target value+. If the search is successful, the new parameter value is set; otherwise, the rule is left unchanged.

\begin{figure}[!htb]
    \centering
    \includegraphics[width=0.5\textwidth]{figures/gui_autotune.png}
    \caption{The automatic parameter tuning configuration pop-up for the ``saliency lower range'' parameter of the Rule 7 behavior function. }
    \label{fig:gui-autotune}
\end{figure}

\subsection{Panel E}
Panel E visualizes specific examples. There are multiple categories of instances to visualize, controlled by the buttons on the top enlarged in Fig.~\ref{fig:gui-E-button}. 

\begin{figure}[!htb]
    \centering
    \includegraphics[width=\textwidth]{figures/gui_E_button.png}
    \caption{Control buttons for instance visualization. }
    \label{fig:gui-E-button}
\end{figure}

The first button decides whether to visualize the whole rule union or only the selected rule. The second button decides whether to visualize every FEU in a sentence or an individual FEU in a sentence. If individual FEUs are visualized, the third button toggles whether to show all FEUs or only the invalid ones. This button is present if the second button is on the ``Sentence'' mode. Finally, the last button refreshes a new batch of examples to present. 

When the second button is set to the ``Sentence'' mode, Fig.~\ref{fig:gui-sentence-mode} shows two example sentences. First, the ground truth and predicted labels are shown, rendered in green for correct prediction and red for incorrect one. Then the sentence is displayed, with the color on each word corresponding to saliency value. The GUI assumes that the values are normalized to the [-1, 1] range, and uses full red for 1 and full blue for -1. An \ul{underline} below the word indicates that it is applicable (by either the rule union or the selected rule, according to the first control button). A \textbf{boldface} on the word indicates that it is valid according to the behavior function. Hovering on each word shows its numeric saliency value and the rule that is effective on it (if any). 

\begin{figure}[!htb]
    \centering
    \includegraphics[width=0.9\textwidth]{figures/gui_sentence_mode.png}
    \caption{Two sentence-mode visualizations, with the mouse cursor hovering over ``an'' on the second sentence. }
    \label{fig:gui-sentence-mode}
\end{figure}

\noindent When the second button is set to the ``FEU'' mode, Fig.~\ref{fig:gui-feu-mode} shows an example sentence. The text coloring follows the same convention. The \ul{underline} signals the specific FEU being visualized. The \textbf{boldface} again indicates the validity. In addition, the predicted behavior range and the actual saliency are shown graphically below each example, as a yellow segment and a dot (green for valid and red for invalid), respectively. 

\begin{figure}[!htb]
    \centering
    \includegraphics[width=0.9\textwidth]{figures/gui_feu_mode.png}
    \caption{Two FEU-mode visualizations. }
    \label{fig:gui-feu-mode}
\end{figure}

\noindent Since the FEU mode conveys much less information than the Sentence mode, this panel also shows a list of behavior range and saliency value visualizations below, without the input text, as shown in Fig.~\ref{fig:gui-bars} (the third button is switched to ``Invalid'' so that all saliency dots are outside of the yellow range and thus red). 

\begin{figure}[!htb]
    \centering
    \includegraphics[width=0.9\textwidth]{figures/gui_bars.png}
    \caption{Additional behavior range visualizations for the FEU mode (shown here are invalid ones only). }
    \label{fig:gui-bars}
\end{figure}

\noindent Last, clicking on each sentence or behavior range bar brings up additional details, as shown in Fig.~\ref{fig:gui-instance-popup}. 

\begin{figure}[!htb]
    \centering
    \includegraphics[width=\textwidth]{figures/gui_instance_popup.png}
    \caption{Detailed information about an example. The four features are: word sentiment score, part of speech, named entity tag, and word frequency. }
    \label{fig:gui-instance-popup}
\end{figure}
